# Supplementary material for: Unsupervised Domain Adaptation for 3D Keypoint Estimation via View Consistency
Source: arXiv:1712.05765 source file (2018-07-26)
Supplement: Supplementary file 1 [file 07_appendix.tex]

\section*{Proof of Prop.~\ref{Prop:2}}
\label{Proof:Prop:2}
Denote $\overline{Y} = R^{T}Y$. Consider the optimal rotation 
$$
R(\overline{X}):= \underset{R}{\textup{argmin}}\ \|\overline{X} - R(\overline{X})^{T}Y\|_{\set{F}}^2.
$$
In the local neighborhood of $X$ (whose corresponding optimal rotation is denoted as $R$), we use the exponential map to parameterize $R(\overline{X})$:
\begin{equation}
R(\overline{X}) = \exp\left(
\begin{array}{ccc}
0 & -c_3(\overline{X}) & c_2(\overline{X}) \\
c_3(\overline{X}) & 0 & -c_1(\overline{X}) \\
-c_2(\overline{X}) & c_1(\overline{X}) & 0 \\
\end{array}
\right)R.
\label{R:parameterization}
\end{equation}
Denote
$$
\overline{X}_i = \bs{e}_i^{T}\overline{X}, \overline{Y}_i = \bs{e}_i^{T}\overline{Y}, \ 1\leq i \leq 3.
$$
Using (\ref{R:parameterization}), we have
\begin{align*}
&\frac{\partial r}{\partial \overline{x}_{ij}}(X,Y)  =    2\langle \overline{X} - \overline{Y}, \frac{\partial \overline{X}}{\partial \overline{x}_{ij}}\rangle \mid_{\overline{X} = X} \\
& -\big((\overline{X}_2 - \overline{Y}_2)^{T}\overline{Y}_3 - (\overline{X}_3 - \overline{Y}_3)^{T}\overline{Y}_2\big)\frac{\partial c_1}{\partial \overline{x}_{ij}}(X) \\
& -\big((\overline{X}_3 - \overline{Y}_3)^{T}\overline{Y}_1 - (\overline{X}_1 - \overline{Y}_1)^{T}\overline{Y}_3\big)\frac{\partial c_2}{\partial \overline{x}_{ij}}(X) \\
& -\big((\overline{X}_1 - \overline{Y}_1)^{T}\overline{Y}_2 - (\overline{X}_2 - \overline{Y}_2)^{T}\overline{Y}_1\big)\frac{\partial c_3}{\partial \overline{x}_{ij}}(X).
\end{align*}
Since $C_i(X) = 0, 1\leq i \leq 3$, we have
\begin{align*}
\big((\overline{X}_2 - \overline{Y}_2)^{T}\overline{Y}_3 - (\overline{X}_3 - \overline{Y}_3)^{T}\overline{Y}_2\big) = 0, \\
\big((\overline{X}_3 - \overline{Y}_3)^{T}\overline{Y}_1 - (\overline{X}_1 - \overline{Y}_1)^{T}\overline{Y}_3\big) = 0, \\
\big((\overline{X}_1 - \overline{Y}_1)^{T}\overline{Y}_2 - (\overline{X}_2 - \overline{Y}_2)^{T}\overline{Y}_1\big) = 0. \\
\end{align*}
This means
$$
\frac{\partial r}{\partial \overline{x}_{ij}}(X,Y) = 2(\overline{x}_{ij}-\overline{y}_{ij}),
$$
which ends the proof.
\qed
